# Supplementary material for: Comparing Video Based Shoulder Surfing with Live Simulation
Source: arXiv:1809.08640 source file (2018-09-23)
Supplement: Supplementary file 1 [file appendix.tex]

% \documentclass[10pt]{article}

% \usepackage{graphicx}
% \usepackage{fullpage}
% \usepackage{times}

% \title{Classifying Eyes-Free Mobile Device Authentication Techniques \\ {\large SUPPLEMENTAL MATERIAL} }
% \date{}

% \begin{document}

% \maketitle

% \section*{List of Provided Material}
% \begin{enumerate}
% \item Visuals of all the PINs and Patterns used in the experiment (see
%   Section~\ref{sec:viz} and {\tt images} sub-directory)
% \item GIFs of classification labels for both the training and authentication
%   (see Section~\ref{sec:class} and {\tt gifs} sub-directory)
% \item Complete survey questions (see Section~\ref{sec:survey})
% \end{enumerate}

% \clearpage

\subsection{Patterns and PINs Visualized}
\label{sec:viz}
\input{pattern_viz}

\subsection{Pre-Survey Questions}

\begin{itemize}
\item What is your age (18-24, 25-34, 35-44, 45-54, +65, NA)?

\item What is your identified gender?

\item Do you have any physical conditions that might affect your ability to
  enter authentication passcodes on a mobile phone?

\item Do you use a smartphone currently? What is its operating system? Why did
  you select that phone?

\item Do you use an authentication method to lock your phone, and if so which
  method, and why (i.e. PIN, grid, TouchID, etc.)?

\item Without telling me your current passcode, how do you select the passcodes
  you use to lock your phone (i.e. familiar number, or visual pattern)?

\item How concerned are you with keeping your phone secure (1, not at all
  concerned, to 5, highly concerned)?  item What experiences can you recall
  involving people either trying to steal or use your phone without permission?

\item What experiences can you recall involving people trying to observe your
  passcodes without permission?

\item How concerned are you, typically, in a public space, with the threat of
  someone watching you authenticate and collecting your passcodes (1, not at all
  concerned, to 5, highly concerned)?

\item If you had any of these experiences, how did it affect your behavior?

\item Have any other experiences or concerns indirectly affected your
  authentication behavior (news articles, stories about friends, etc.)?

\item If you do authentication, how do you typically hold your phone for that?

\end{itemize}

\subsection{Post-Survey Questions}
\begin{itemize}
\item On a scale from 1-5, how difficult was entering passcode this way (1, very
  easy, to 5, very hard)? How so?

\item On a scale from 1-5, how easy was the grid pattern tactile app to learn
  (1, very easy, to 5, very hard)? How so?

\item On a scale from 1-5, how easy was the grid pattern tactile app to use (1,
  very easy, to 5, very hard)? How so?

\item On a scale from 1-5, how easy was the PIN tactile app to learn (1, very
  easy, to 5, very hard)? How so?

\item On a scale from 1-5, how easy was the PIN tactile app to use (1, very
  easy, to 5, very hard)? How so?

\item Can you see yourself using the grid pattern tactile aid to help
  authenticate on your phone in your actual daily life? Why or why not?

\item Can you see yourself using the PIN tactile aid to help authenticate on
  your phone in your actual daily life? Why or why not?

\item How is this approach similar or different from how you enter passcodes on
  your phone now?

\item Do you think the grid tactile aid would help protect you from someone
  shoulder surfing you? Why or why not?

\item Do you think the PIN tactile aid would help protect you from someone
  shoulder surfing you? Why or why not?

\end{itemize}

%%% Local Variables:
%%% mode: latex
%%% TeX-master: "main"
%%% End:
